# Supplementary material for: Geometric Resonance of Four-Flux Composite Fermions
Source: arXiv:1907.07563 ancillary file (2019-07-29)
Supplement: Supplementary file 1 [file Supplemental_Materials_Shafayat_FourfluxCF.pdf]

# Supplemental materials: Geometric resonance of four-flux composite fermions

Md. Shafayat Hossain,<sup>1</sup> Meng K. Ma,<sup>1</sup> M. A. Mueed,<sup>1</sup> D. Kamburov,<sup>1</sup> L. N. Pfeiffer,<sup>1</sup> K. W. West,<sup>1</sup> K. W. Baldwin,<sup>1</sup> R. Winkler,<sup>2</sup> and M. Shayegan<sup>1</sup>

<sup>1</sup>*Department of Electrical Engineering, Princeton University, Princeton, New Jersey 08544, USA*

<sup>2</sup>*Department of Physics, Northern Illinois University, DeKalb, Illinois 60115, USA*

(Dated: July 12, 2019)

## I. EXPERIMENTAL DETAILS

Our sample is a low-disorder two-dimensional electron system (2DES) with density  $n = 1.78 \times 10^{11} \text{ cm}^{-2}$  and low-temperature mobility  $1.4 \times 10^7 \text{ cm}^2/\text{Vs}$ . The 2DES is confined to a modulation-doped, 40-nm-wide, GaAs quantum well, flanked by 190-nm-thick  $\text{Al}_{0.30}\text{Ga}_{0.70}\text{As}$  barrier (spacer) layers, all grown via molecular beam epitaxy on a (001) GaAs substrate. The 2DES is buried 235 nm underneath the surface. The sample structure is illustrated in Fig. S1(a). For our measurements, L-shaped Hall bar samples were fabricated using standard photolithography techniques. The sample comprises multiple sections, each of length  $100 \mu\text{m}$  and width  $50 \mu\text{m}$ , as shown in the inset of Fig. 1(b) of the main text. Via electron-beam lithography and using a calixarene-based negative electron-beam resist, we patterned the surface with strain-inducing superlattices of period  $a = 240 \text{ nm}$  perpendicular to the current direction. A scanning electron micrograph of such a superlattice is shown in Fig. S1(b). The L-shaped Hall bar enables us to perform geometric resonance (GR) measurements along two perpendicular crystallographic directions,  $[110]$  and  $[\bar{1}10]$ . These measurements of GR along the two perpendicular directions are used to extract the anisotropy of the CF Fermi contour.

The measurements were done in a dilution refrigerator with a base temperature of 50 mK via passing current ( $I = 1\text{--}10 \text{ nA}$ , 13 Hz) perpendicular to the density modulation. The experiments were performed using the 45 T hybrid magnet facility at the National High Magnetic Field Laboratory, Tallahassee, Florida.

The low-temperature mobility of our sample,  $1.4 \times 10^7 \text{ cm}^2/\text{Vs}$ , is very high and therefore favorable to ballistic transport of composite fermions (CFs). This is a necessary condition for observing the GR features. Figures S2(a-d) present the magneto-resistance traces in a patterned section ( $a = 240 \text{ nm}$ ) of the Hall bar, zooming in around  $\nu = 3/2$ ,  $1/2$ ,  $3/4$ , and  $1/4$  CF seas, respectively. They exhibit GR features flanking the V-shaped minima. Green dashed lines mark the expected positions of the primary GR features assuming a fully spin-polarized CF sea. The GR minima around  $\nu = 1/2$ ,  $3/4$ , and  $1/4$  are in excellent agreement with such an assumption of full spin-polarization. The GR minima around  $\nu = 3/2$ , on the other hand, are nearer to the V-shaped minimum at

$\nu = 3/2$  compared to the expected positions for the fully spin-polarized CFs. This indicates that the CFs around  $\nu = 3/2$  are not fully spin-polarized, consistent with the findings of Ref. [42] of the main text.

One important aspect of these data is the observation of the GR features around  $\nu = 3/4$ . Even though the features are very weak, this is the first observation of a CF sea around  $\nu = 3/4$ . The positions of the GR minima around  $\nu = 3/4$  suggest a fully spin-polarized four-flux CF ( $^4\text{CF}$ ) Fermi sea near  $\nu = 3/4$ .

## II. ADDITIONAL DATA AND DISCUSSIONS

In this section, first, we show an extended data set for the tilt evolution of the  $^4\text{CF}$ s near  $\nu = 1/4$ . We show a limited portion of this data in Fig. 2 of the main text. Magneto-resistance traces for the two arms of our L-shaped Hall bar along the  $[110]$  and  $[\bar{1}10]$  directions are shown in Figs. S3(a) and S3(b). In both panels, the vertical green dotted lines mark the expected positions of the  $i = 1$   $^4\text{CF}$  GR minima based on fully spin-polarized  $^4\text{CF}$ s with circular Fermi contours, i.e.,  $B_{i=1}^* = 2\hbar\sqrt{4\pi n}/ea(1 + 1/4)$ . These lines match reasonably well with the observed positions of the resistance minima for the bottom traces of Fig. S3, which were taken at  $\theta = 0^\circ$  ( $B_{\parallel} = 0$ ). When we increase  $\theta$  and thereby  $B_{\parallel}$ , for the  $[110]$  arm [Fig. S3(a)], the positions of the two GR minima shift away from the dashed lines to higher values of  $|B_{\perp}^*|$ . In contrast, the GR minima for the arm along  $[\bar{1}10]$  direction [Fig. S3(b)] move towards lower  $|B_{\perp}^*|$ .

In Fig. S4 we show additional  $^4\text{CF}$  GR data for two other 40-nm-wide GaAs quantum well samples with two different densities,  $n = 1.74 \times 10^{11} \text{ cm}^{-2}$  (sample A) and  $0.91 \times 10^{11} \text{ cm}^{-2}$  (sample B). The structures of these samples are slightly different from the sample used in the main text and the previous section. Consequently, the superlattice periods that are required to observe clear  $^4\text{CF}$  GR are also different. Note that, the period of the superlattice required to observe clear GR features depends on the electron density and the depth of the 2DES from the surface. In sample A, the 2DES is 190 nm underneath the surface. Therefore, we use a superlattice period of  $a = 200 \text{ nm}$  for an appropriate modulation. On the other hand, sample B contains a 2DES that is 235 nm underneath the surface. Since the electron density

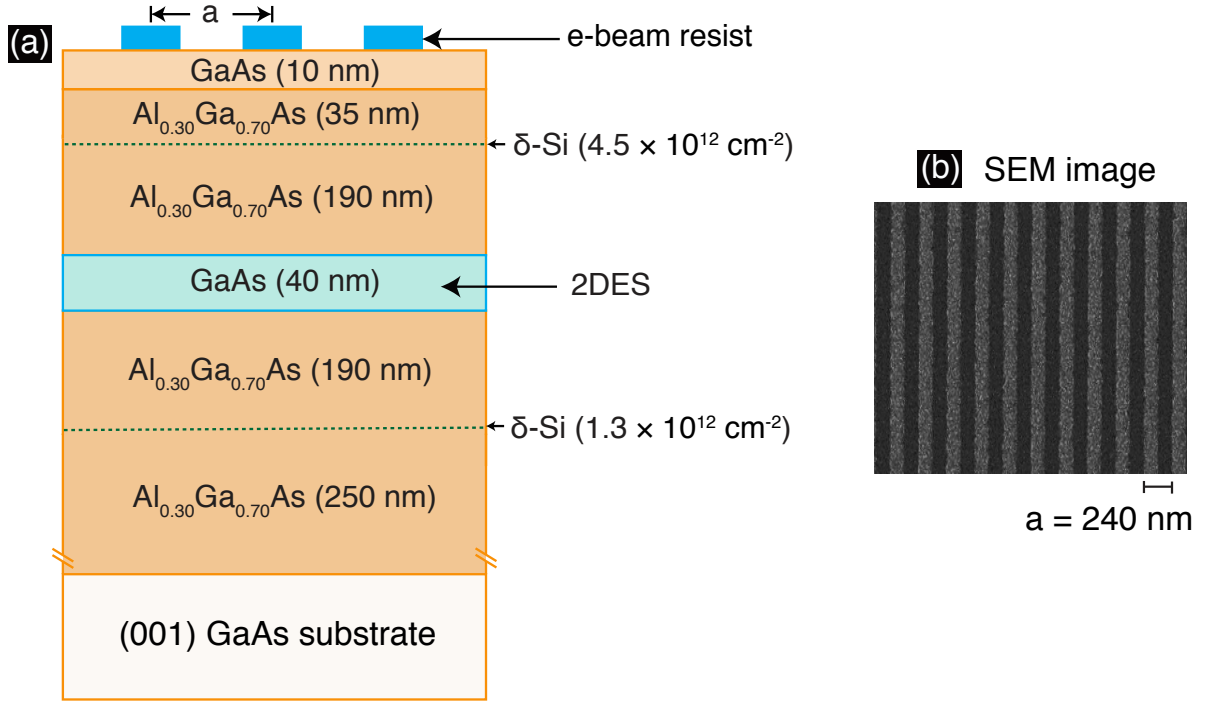

FIG. S1. (a) The structure of the studied GaAs quantum well sample. The quantum well is flanked by 190-nm-thick  $\text{Al}_{0.30}\text{Ga}_{0.70}\text{As}$  spacer layers to ensure a good quality 2DES which supports the ballistic transport of composite fermions. (b) The scanning electron microscope (SEM) micrograph of a 240-nm-patterned section attests to the uniformity of the stripes in the superlattice.

is much lower in sample B, we find a superlattice with  $a = 225$  nm to be optimum for obtaining clear GR features. The measurements were taken at  $T = 0.3$  K using a  $^3\text{He}$  cryostat.

In Figs. S4(a) and S4(b) the traces show a rising, linear, background resistance on the low-filling side of  $\nu = 1/4$ . This is especially prominent in the sample with lower density [Fig. S4(b)]. Therefore, we perform a linear background subtraction before extracting the field positions of the  $^4\text{CF}$  GR features for these traces. Figures S4(c) and (e) show the unprocessed data while Figs. S4(d) and (f) exhibit the trace after the subtraction. Similar to the main text, we mark the expected positions for the  $i = 1$   $^4\text{CF}$  GR in Figs. S4(c-f) considering two possibilities: (i) black solid lines for  $k_F^* = \sqrt{4\pi n}$ , and (ii) orange dashed lines for  $k_F^*$  changing according to the magnetic length, i.e.,  $k_F^* = \sqrt{4\pi n} \times \sqrt{B/B_{\nu=1/4}}$ . In both cases, we assume that the  $^4\text{CFs}$  are fully spin-polarized. Again, we find that the difference between the expected  $B_{i=1}$  for the two assumptions is very small and cannot be resolved in our experiments. Similar to Fig. 1(c), here

we also find that the observed GR minima positions are in excellent agreement with the expected  $B_{i=1}$ . These data further corroborate our observations described in the main text that there is no noticeable asymmetry in the field positions of the GR minima flanking  $\nu = 1/4$  when  $B_{||} = 0$  (Fig. 1).

The background resistance rise at high magnetic fields in Figs. S4(a) and S4(b) likely stems from the proximity of the pinned Wigner crystal formation at low fillings which is known to manifest as an insulating phase starting around  $\nu \simeq 0.21$  (see Refs. [30, 31, 33, 34] of main text). It is noteworthy that the magneto-resistance traces of Figs. S4(a) and S4(b), including the positions and shapes of the  $^4\text{CF}$  GR minima for  $\nu > 1/4$  appear to be unaffected by the proximity of the Wigner crystal. The resistance rise which also affects the shape of the GR minima significantly in Figs. S4(a) and S4(b) indeed appears to suddenly set in once  $\nu$  becomes smaller than  $1/4$ . This is surprising, and suggests that something special happens to the ground state of the 2DES once  $\nu < 1/4$  is reached.

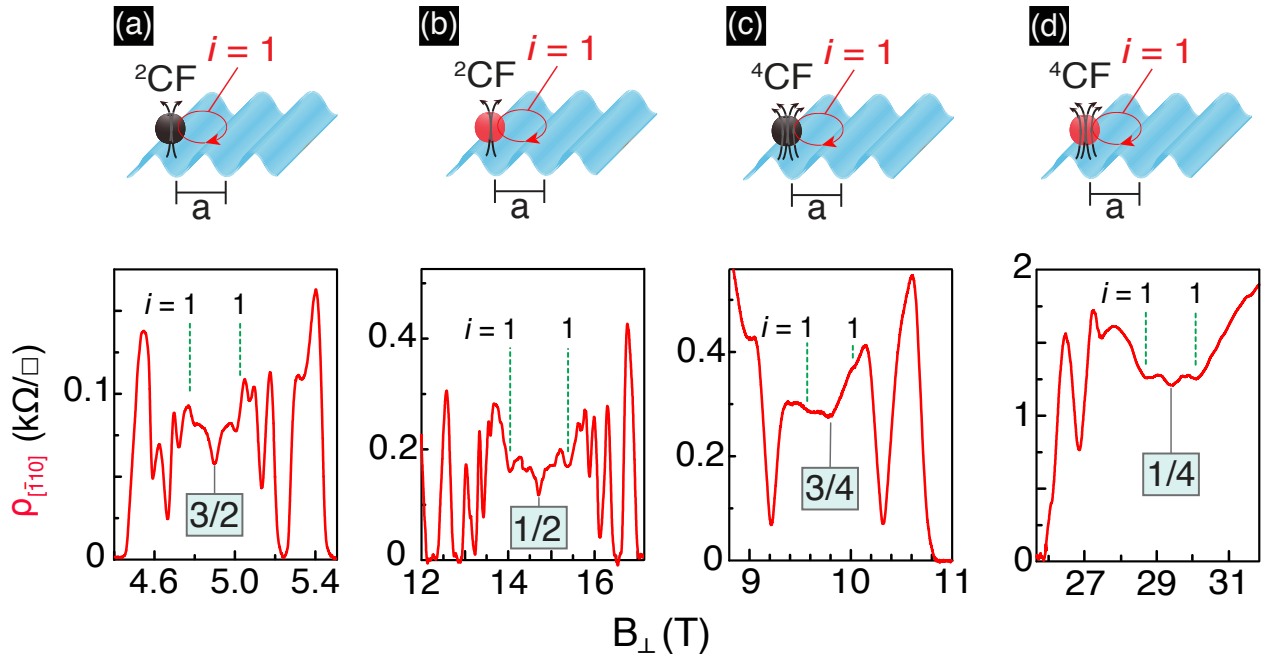

FIG. S2. CF GR features for two- and four-flux CFs in our sample with  $n = 1.78 \times 10^{11} \text{ cm}^{-2}$  and superlattice period  $a = 240 \text{ nm}$ . Traces were taken at  $T \simeq 0.18 \text{ K}$ . (a) and (b) show the GR features of the two-flux CFs ( $^2\text{CFs}$ ) around  $\nu = 3/2$  and  $1/2$ , respectively. (c) and (d) depict the GR features of four-flux CFs ( $^4\text{CFs}$ ) around  $\nu = 3/4$  and  $1/4$ , respectively. Vertical dotted lines mark the expected positions for the primary GR features assuming that the CFs are fully spin-polarized.

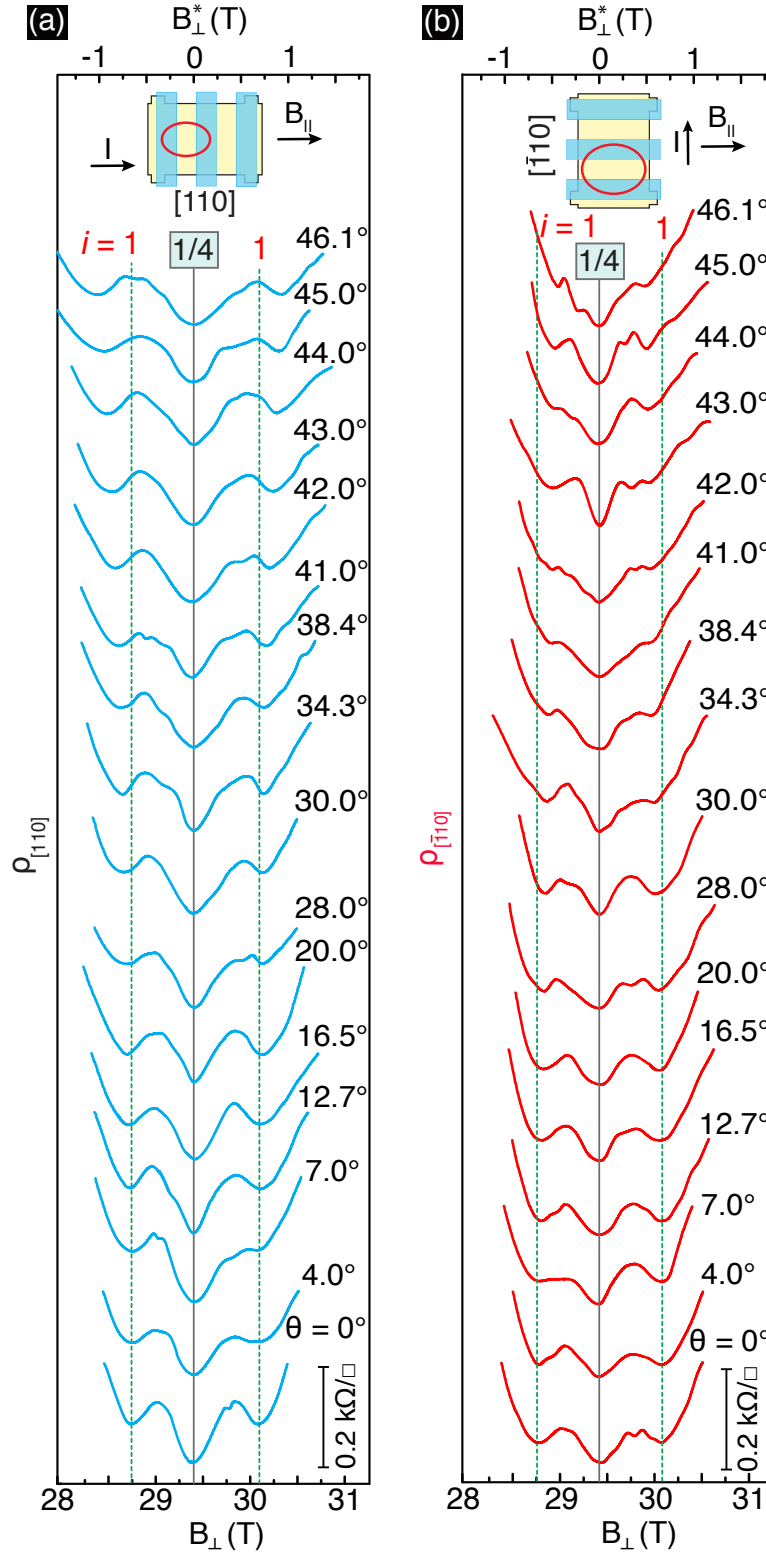

FIG. S3. Tilt evolution of the  ${}^4\text{CF}$  GR features near the  $\nu = 1/4$  along (a)  $[110]$  and (b)  $[\bar{1}10]$  directions. All the traces were taken at  $T \simeq 0.18 \text{ K}$ . The insets show the orientation of the Hall bars, and the  ${}^4\text{CF}$  cyclotron orbit for the  $i = 1$  GR. The direction of the in-plane field ( $B_\parallel$ ) is  $[110]$ . The *expected* positions for primary  $i = 1$   ${}^4\text{CF}$  GRs are marked with dotted lines assuming that the  ${}^4\text{CF}$ s are fully spin-polarized and their cyclotron orbit is circular. In both panels, the scale for the applied external magnetic field  $B_\perp$  is shown on bottom while the top scale is the effective magnetic field  $B_\perp^*$  experienced by the  ${}^4\text{CF}$ s. In some traces, there are extra features between the V-shaped minimum at  $\nu = 1/4$  and the primary  $i = 1$   ${}^4\text{CF}$  GR. They very likely stem from the second-order ( $i = 2$ ) GR.

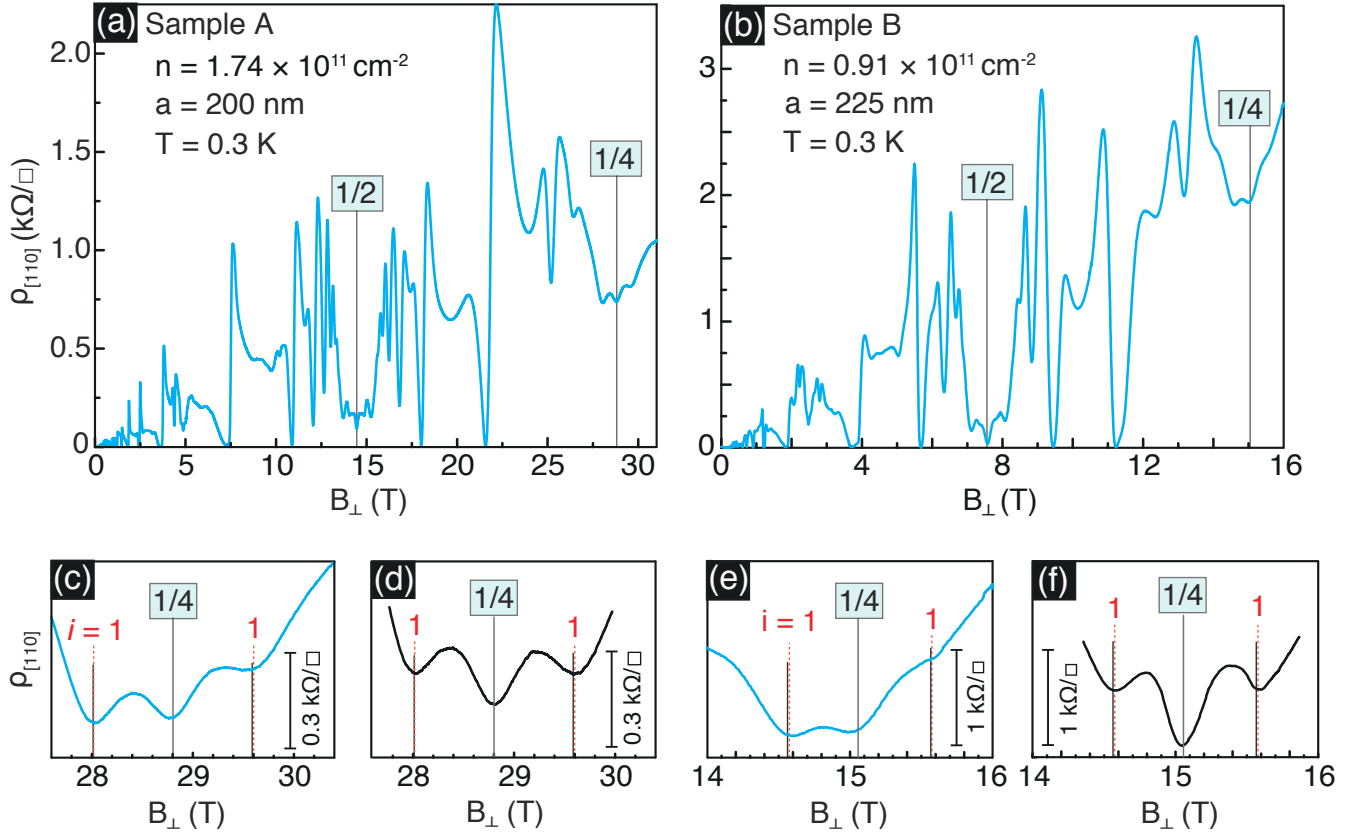

FIG. S4. (a) and (b) Magneto-resistance traces measured at  $T = 0.3$  K for two other 40-nm-wide quantum well samples of densities  $n = 1.74 \times 10^{11} \text{ cm}^{-2}$  (sample A) and  $0.91 \times 10^{11} \text{ cm}^{-2}$  (sample B), respectively. For the sample A, the superlattice period is  $a = 200$  nm and for the sample B, the period is 225 nm. Note that the period is chosen according to the depth of the 2DES from the surface in order to achieve the required modulation strength (see text). (c) and (e) show a zoomed-in magneto-resistance trace around  $\nu = 1/4$  exhibiting GR features of  $^4$ CFs in the form of resistance minima flanking the V-shaped minima at  $\nu = 1/4$ . (d) and (f) depict the traces after subtracting a linear background from the traces shown in (c) and (e), respectively. Black solid lines and orange dotted lines mark the *expected* positions for the  $i = 1$  GR for fully spin-polarized  $^4$ CFs with a circular Fermi sea assuming  $k_F^* = \sqrt{4\pi n}$  and  $k_F^* = \sqrt{4\pi n} \times \sqrt{B/B_{\nu=1/4}}$ , respectively.
